# Supplementary material for: Towards cost-effective and resource-aware aggregation at Edge for Federated Learning
Source: arXiv:2204.07767 source file (2024-01-27)
Supplement: Supplementary file 1 [file Appendix.tex]

\mysection{Identifying Bottlenecks in Current Aggregation Strategies}
\label{Identifying_Bottlenecks_in_Current_Aggregation_Strategies}

The performance of the aggregator server during the FL process is affected by the use of various resources such as CPU, memory, and network. To identify the bottlenecks in the aggregation process and make informed design choices, it is important to empirically examine the strengths and weaknesses of different design choices. We aim to provide an in-depth analysis of these design choices by examining the common basic operations of various fusion algorithms. Our analysis will also provide key insights that can be used to design an aggregator that can adapt to changing circumstances and optimize its utility under limited resources.

\textbf{Our experiment setup is as follows}. The node has 64 cores Intel(R) Xeon(R) Gold 6226R CPU @ 2.90GHz, 12 Micron DIMM DDR4 Synchronous Registered Memory @ 3200 MHz, network interface as Intel Ethernet Controller 10G X550T with 10Gbit/s dual ports capacity and 256 GB total memory. We test current state-of-the-art FL fusion algorithms Federated averaging (FedAvg) and Iterative averaging (IterAvg) with the IBM Federated Learning Library (IBMFL version 1.0.6) \cite{ludwig2020ibm} that uses Numpy \cite{harris2020arraynumpy}. We chose to use IBMFL for our study because it is a research tool that is also widely used in the industry. IBMFL provides support for various fusion algorithms that are suitable for aggregation purposes. FedAvg and IterAvg are based on averaging and it is the \textbf{common basic operation} of most fusion algorithms such as ClippedAveraging and ConditionalThresholdAveraging in \cite{reina2021openfl} and FedAvg, IterAvg, Gradient Aggregation fusion algorithms in~\cite{ludwig2020ibm}. We sample five percent of clients per round from the total available clients for all our experiments. \looseness=-1

\begin{figure}
%\vspace{-20pt}
\centering
\centerline{\includegraphics[width=1.0\columnwidth]{ 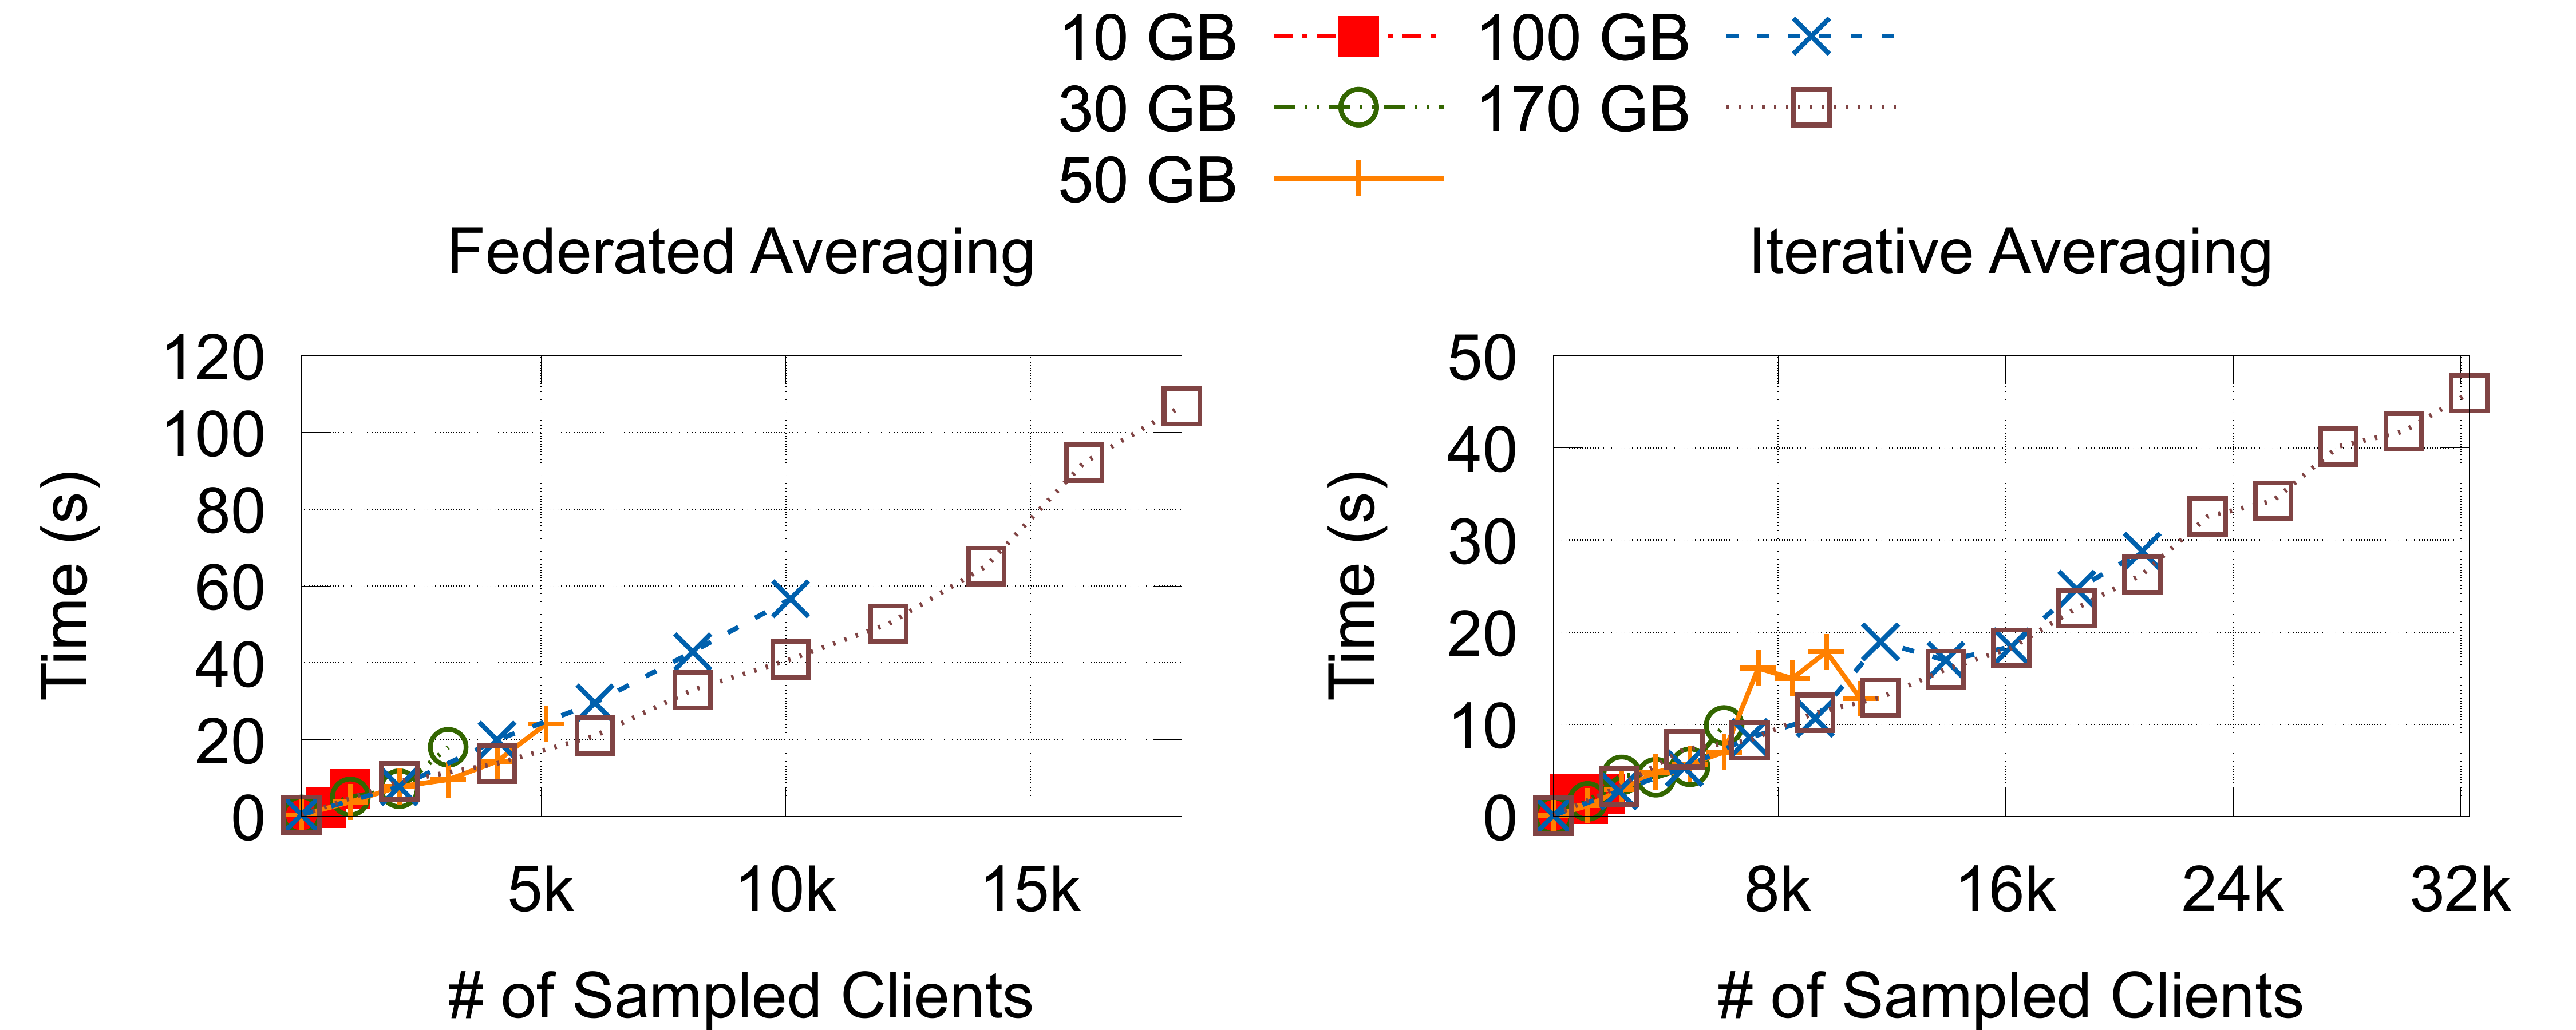}}
\vspace{-1.0em}
\caption{Average aggregation time for IBMFL under different memory capacities for Iteravg and Fedavg algorithms}
\label{fig:vanilla_aggregation_diff_memory}
\vspace{-15pt}
\end{figure}

\begin{figure}
%\vspace{-1.0em}
% \centering
\centerline{\includegraphics[width=0.7\columnwidth]{ 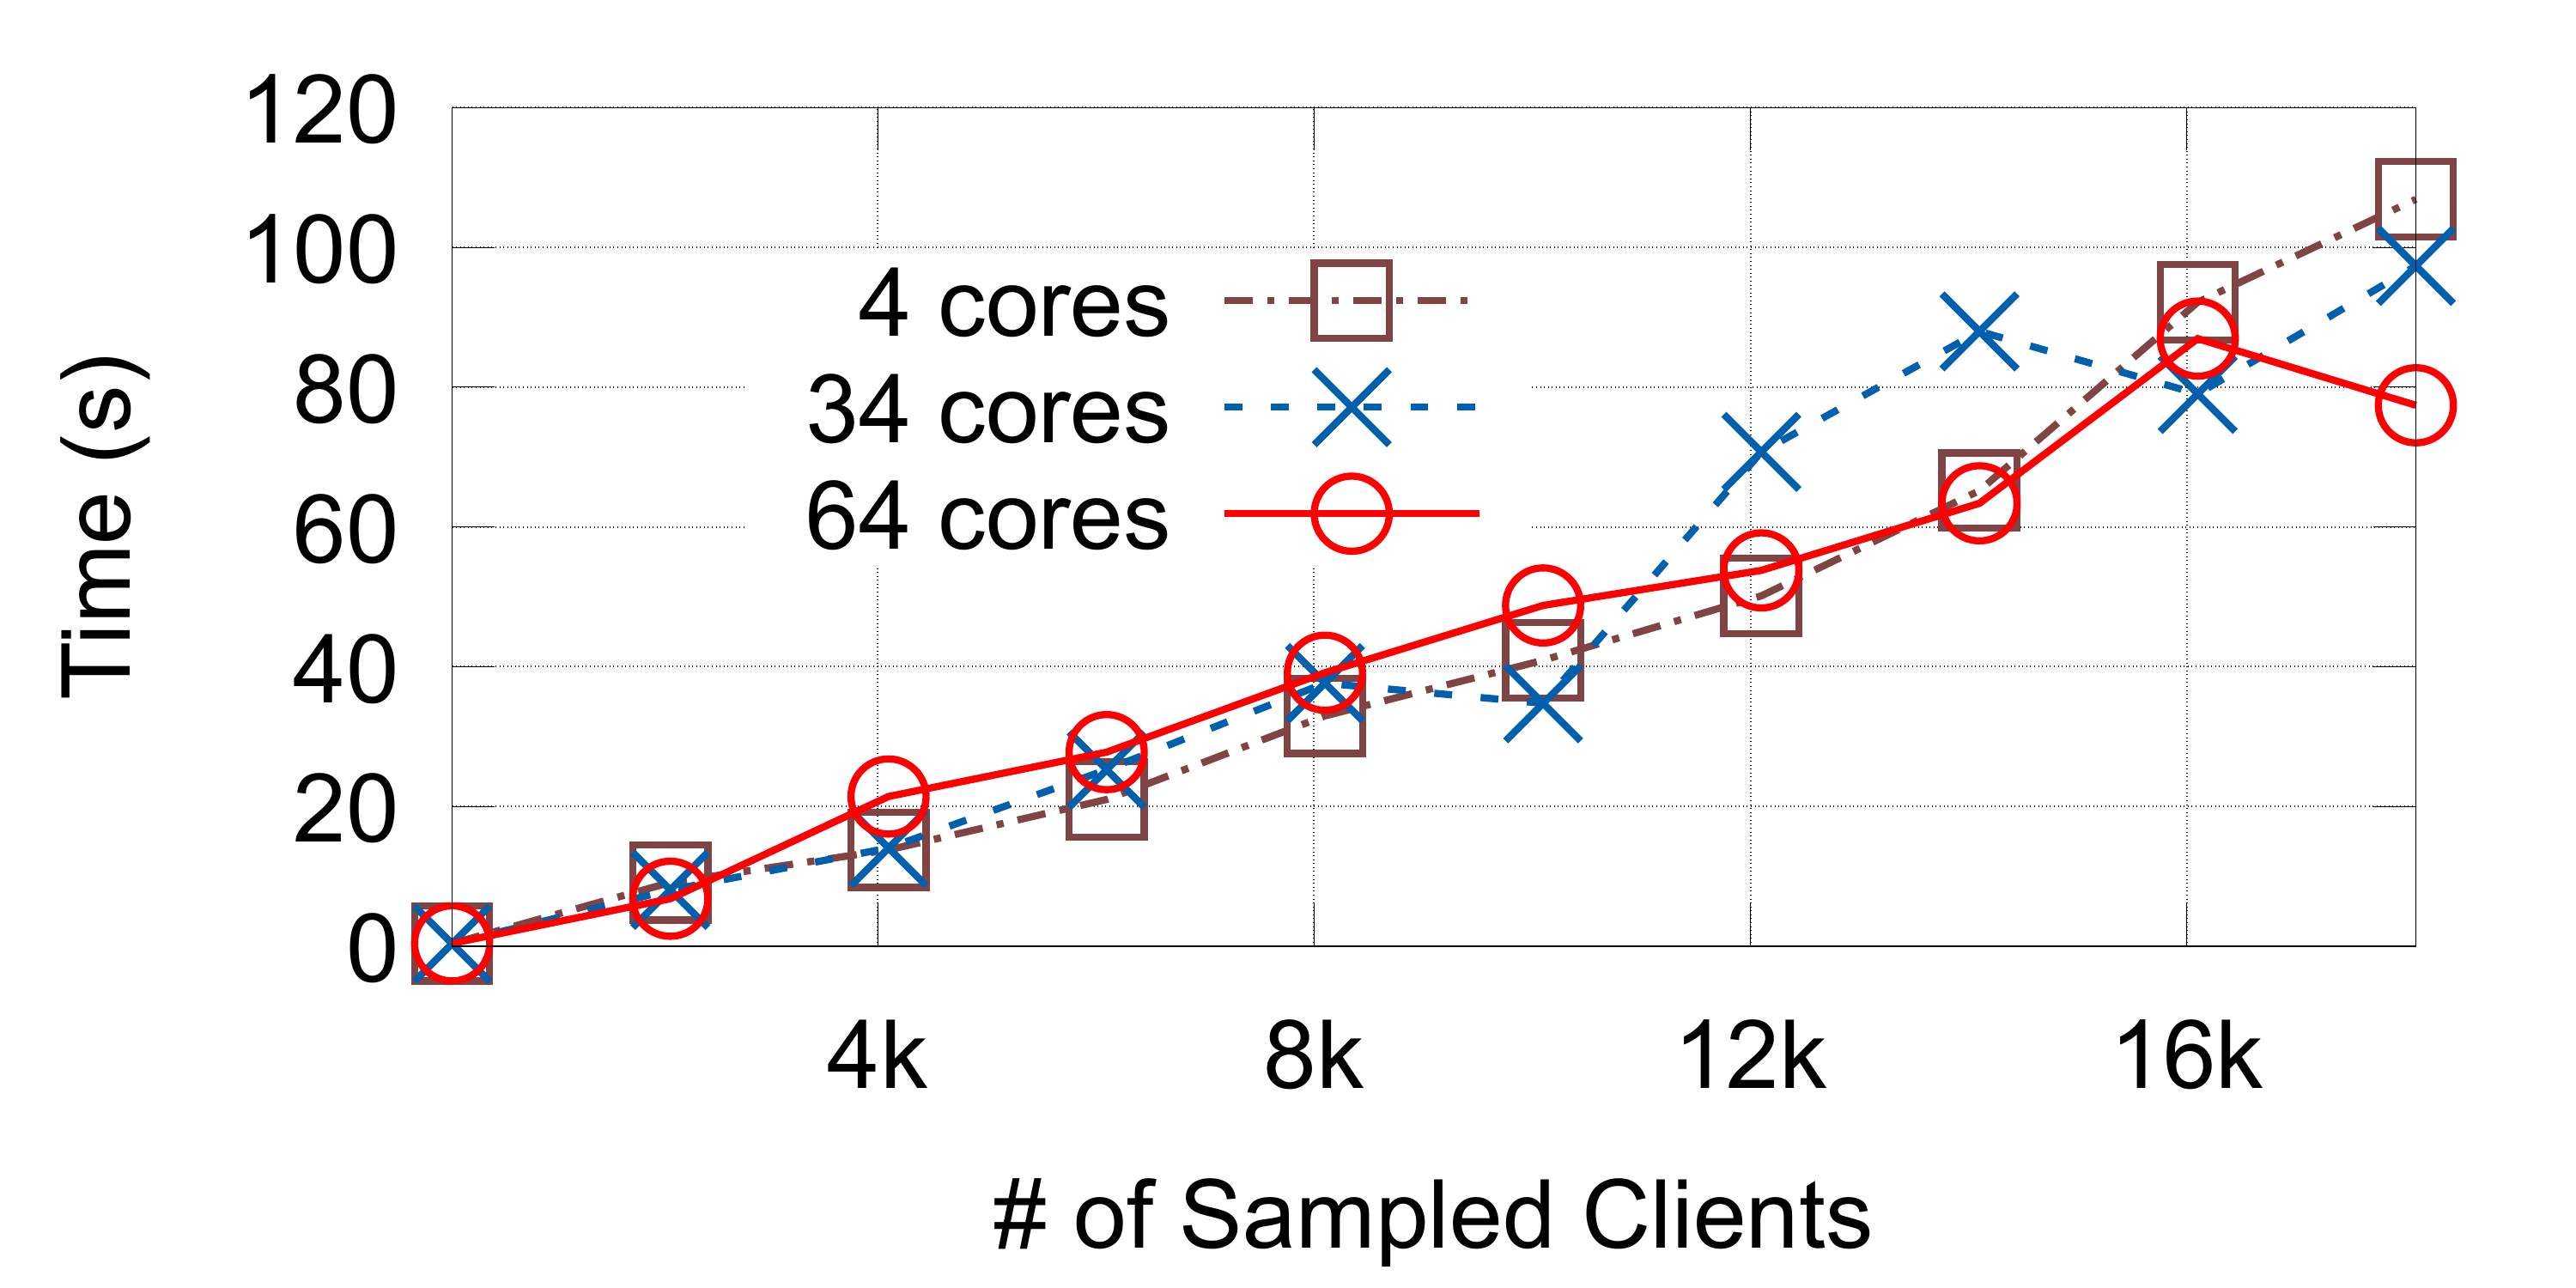}}
\vspace{-5pt}
\caption{Average aggregation time for IBMFL Fedavg algorithm under 170 GB total available memory with different numbers of CPU cores}
\label{fedavg_diff_cores}
\vspace{-1.0em}
\end{figure}

\begin{figure}
%\vspace{-5pt}
\centering
\centerline{\includegraphics[width=1.0\columnwidth]{ 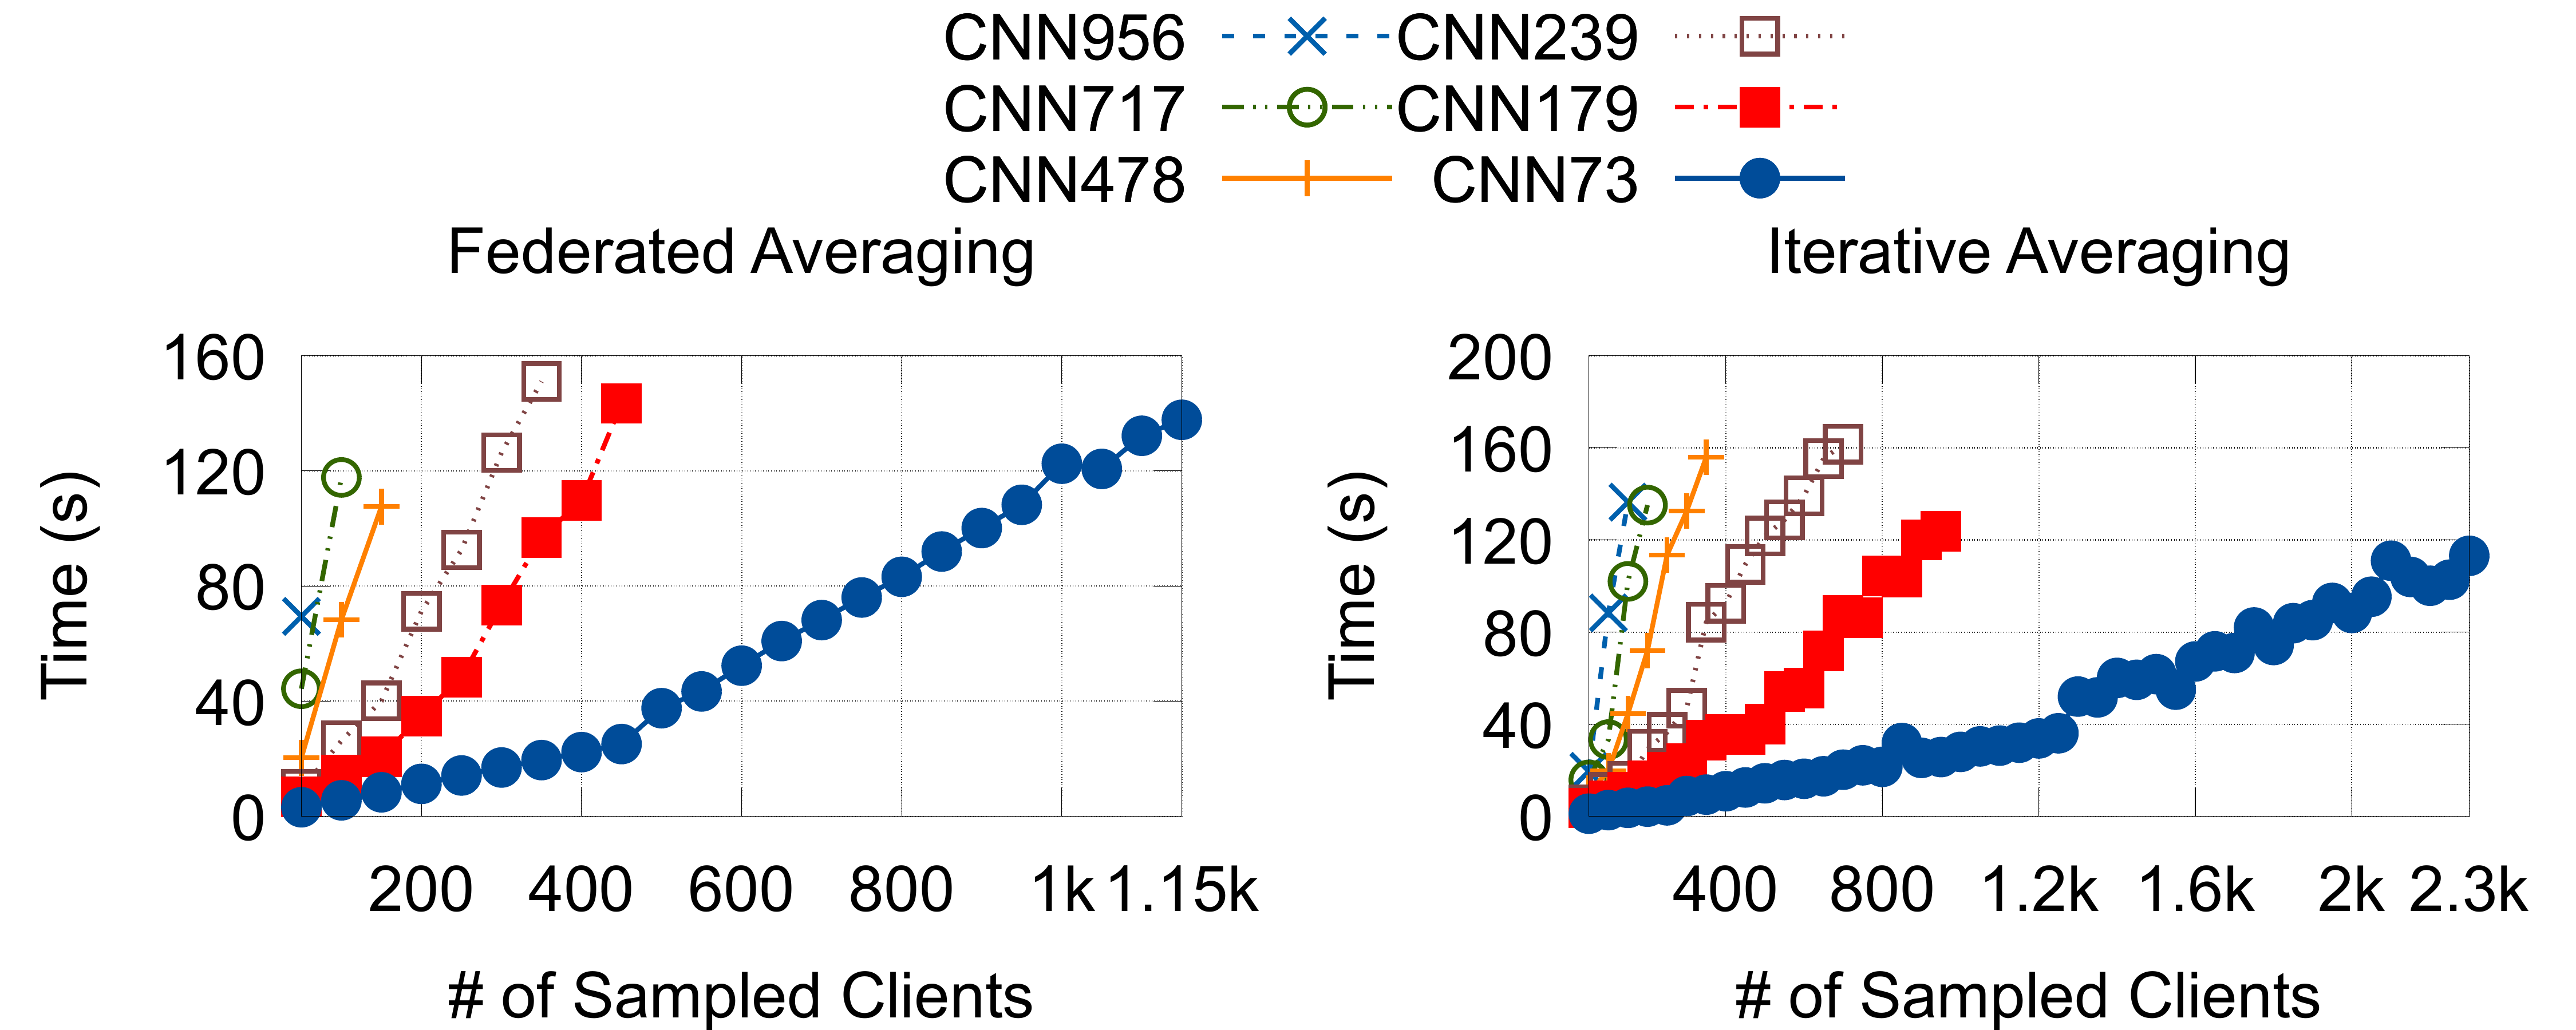}}
\caption{Average aggregation time for IBMFL with varying model sizes without model compression under 170 GB total available memory}
\label{fig:vanilla_aggregation_diff_models_no_compressed}
\vspace{-15pt}
\end{figure}

\mysubsection{Memory Resource Constraint Analysis}
\label{subsec:MemoryResourceConstraintAnalysis}
Our study examines how restricted memory impacts the aggregation process in FL. The amount of memory used is dependent on the number of clients and the size of the model, which can change dynamically. We hypothesize that limited memory will have two effects: 1) the aggregator will only be able to process a limited amount of client data, and 2) the number of clients that the aggregator can support will be correlated with the size of the model.

To test our hypothesis, we conducted controlled experiments with stable CPU resources, incrementally adjusting the total available memory and the number of selected clients.
% The CPU resources (64 cores Intel(R) Xeon(R) Gold 6226R CPU @ 2.90GHz) of the single server are kept constant.

% \end{center}

To evaluate the performance of the aggregation process in FL, we use the CNN4.6 model, which is described in Table \ref{table:benchmarks}. We exclude the time required for data loading by IBMFL when measuring the wall-clock time needed to perform the average for different memory capacities and the number of supported clients. Figure \ref{fig:vanilla_aggregation_diff_memory} summarizes the results. We find that the maximum number of clients that can be supported for aggregation with 170 GB of memory is 18,900 for Federated Averaging (FedAvg) and 32,400 for Iterative Averaging (IterAvg). Beyond these limits, the system runs out of memory. With lower system memory, the limit is reached even more quickly. Our findings demonstrate that scalability in aggregation on a single node is heavily constrained by memory capacity, and the maximum number of supported clients depends on the memory footprint of the fusion algorithm. Specifically, FedAvg can only support up to 20,000 clients, whereas IterAvg can support up to 32,000 clients with 170 GB of memory.

\mysubsection{Impact of limited compute resources}
\label{subsec:CPUResourceConstraintAnalysis}
To assess the limitations of the aggregator architectures in open-source FL frameworks \cite{ludwig2020ibm, TnsorFlowFederated}, we conducted an experimental study using the same configurations and settings as in the previous section. As depicted in Figure \ref{fedavg_diff_cores}, our results indicate that increasing the number of available CPU cores does not have a significant impact on execution time because these frameworks rely on Numpy, which does not support multi-core computation by default. However, to address this issue, we evaluate a multi-core approach in Section \ref{Multi Core}. Our preliminary findings suggest that current FL frameworks~\cite{ludwig2020ibm, reina2021openfl, microsoftFLUTE} are not effectively utilizing system resources, resulting in reduced scalability and efficiency at increased costs.

\mysubsection{Impact of aggregation workloads}
\label{ModelSizeConstraintAnalysis}
To evaluate the aggregator server's ability to handle various model sizes, as discussed in Section \ref{OverviewofExistingAggregationStrategies}, we perform an experiment similar to the one in Section \ref{subsec:MemoryResourceConstraintAnalysis} on a single server with 170 GB of total memory and 64 cores. Additionally, we test the impact of compression of the model, a feature offered by frameworks like IBMFL \cite{ludwig2020ibm} that reduces communication costs between clients and the server. Communication cost reduction is essential for IoT and Edge devices~\cite{IoT_challenges, iot_challenges_compute, iot_challenges_energy} with limited network capacity. We present results with both compressed and uncompressed updates.

\emph{Without compression}, as shown in Figure \ref{fig:vanilla_aggregation_diff_models_no_compressed}, the experiment's results indicate that the time required to perform the weighted average calculation increases as the model size increases, and fewer clients can be supported. With the CNN956 model, we found that less than 150 clients could be supported.

\begin{figure}
%\vspace{-5pt}
\centering
\centerline{\includegraphics[width=1.0\columnwidth]{ 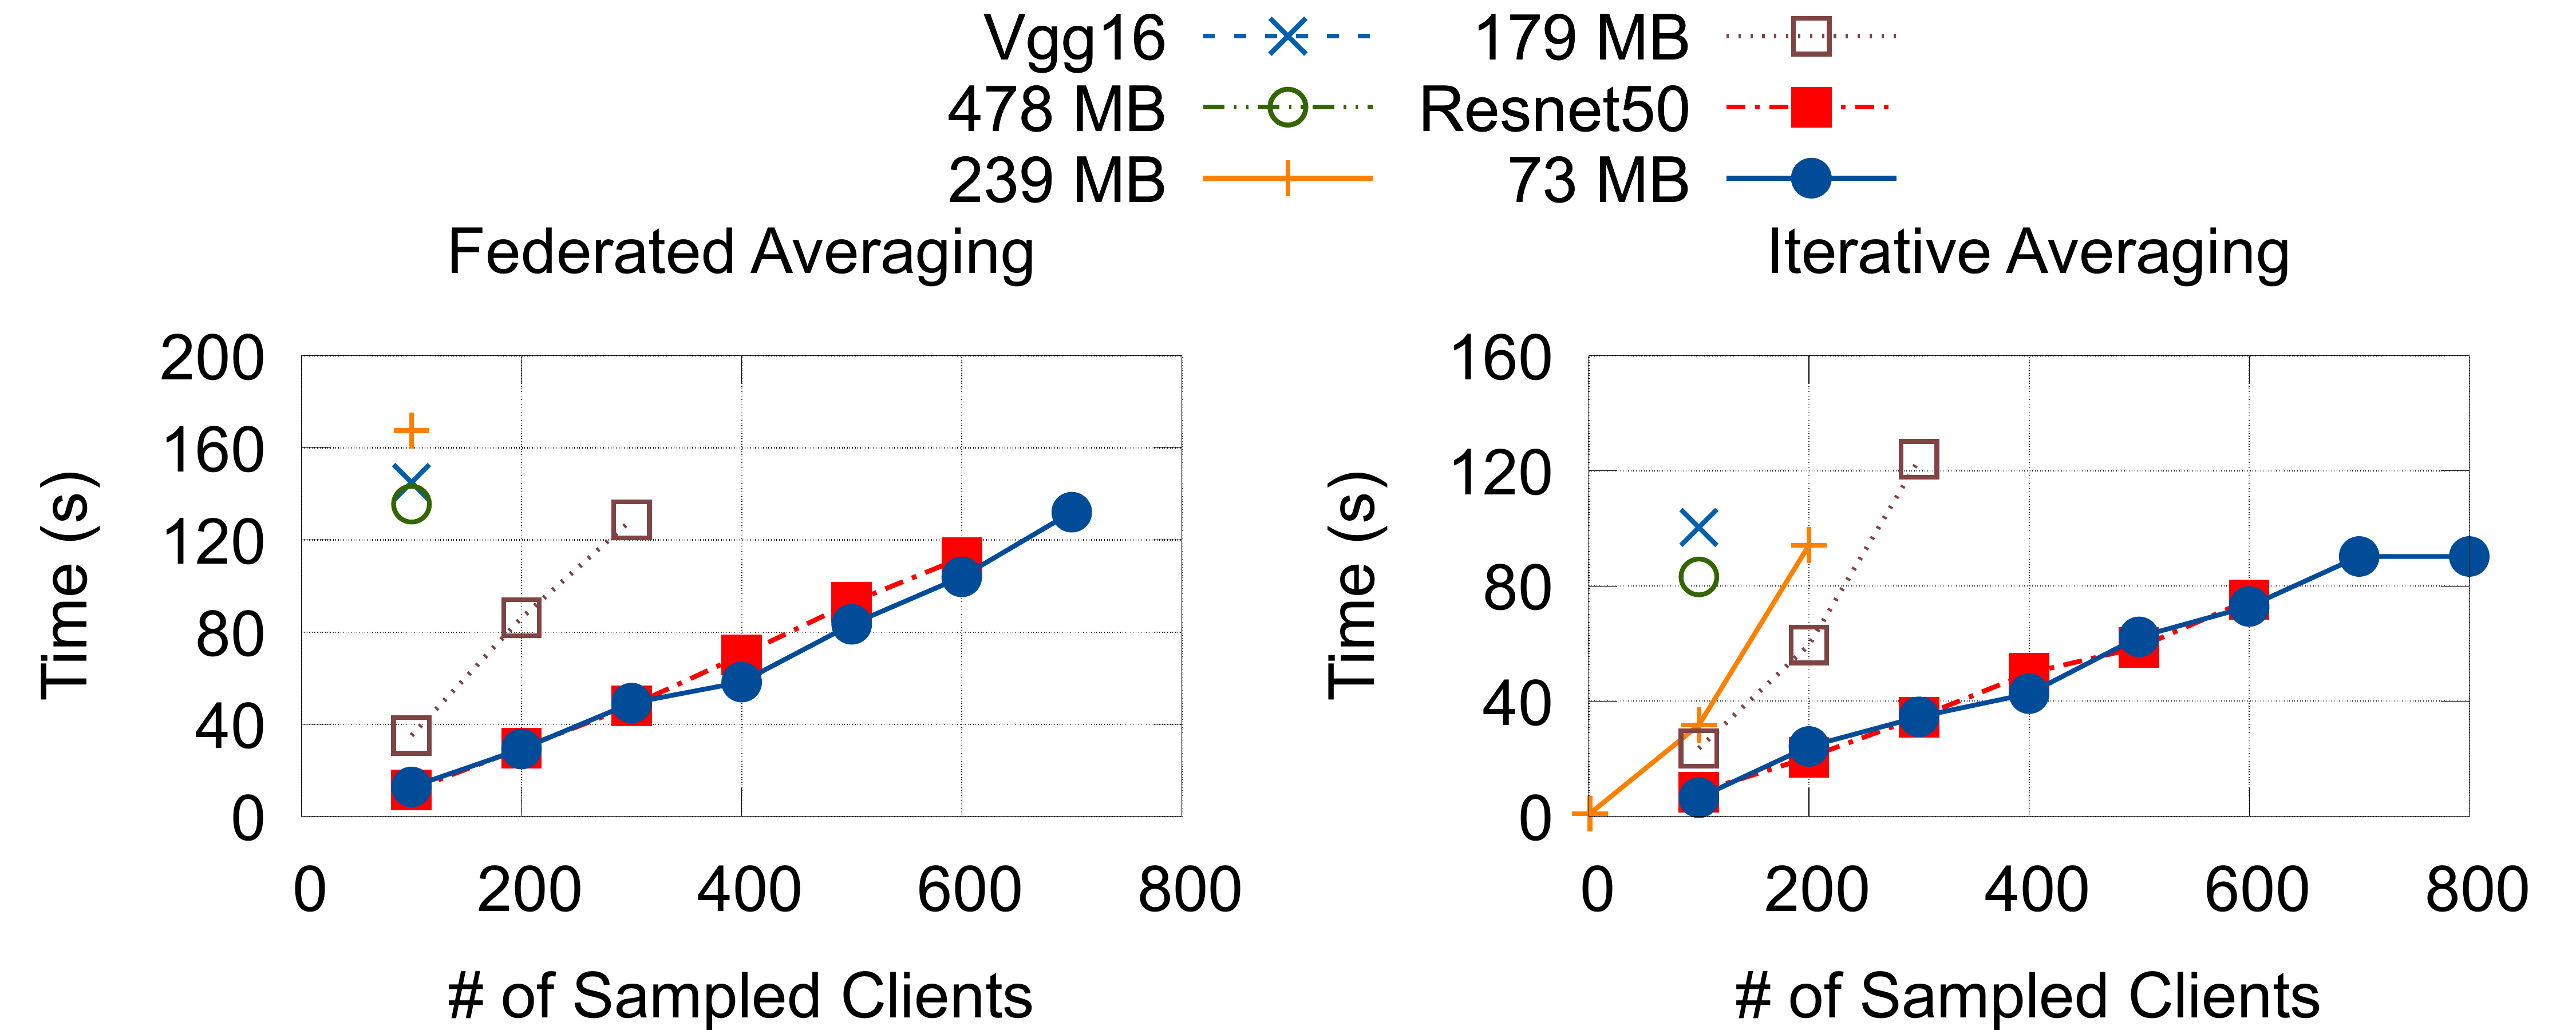}}
\vspace{-10pt}
\caption{Average aggregation time for IBMFL with varying model sizes with compression under 170 GB of total available memory}
\label{fig:vanilla_aggregation_diff_models_compressed}
\vspace{-20pt}
\end{figure}

\emph{With compression:} When compression is applied to the model updates before they are sent to the aggregator, it increases the compute and memory burden on the aggregator. This is because the aggregator not only needs to receive the updates in memory but also needs to decompress them within the same memory capacity, which is already occupied by the compressed updates. The results of this analysis are shown in Figure \ref{fig:vanilla_aggregation_diff_models_compressed}. This approach does not scale well, and fewer clients can be supported for VGG16 aggregation compared to CNN956, with the number of supported clients being less than 150 for VGG16, which is smaller than CNN956 by 428MB.

While the compression and decompression process can be streamlined to avoid memory occupation of compressed data once it has been decompressed, this will further add to the computational costs. We analyze both with and without compression to draw useful trends. Figures \ref{fig:vanilla_aggregation_diff_models_no_compressed} and \ref{fig:vanilla_aggregation_diff_models_compressed} show that compute resources become a bottleneck when the model size increases, leading to reduced time efficiency. 

\mysection{Other Multi-node Tools}
\label{Other distributed methodologies}
A comparison of Dask to the Spark-based method using the Fedavg fusion algorithm in figure \ref{fig:dask_pyspark_resnet50} shows that Dask performed less efficiently than Spark due to spending more time on I/O and conversion to its native Bag type. Spark offers better read-and-write throughput with cloud storage and efficiently partitions data for MapReduce computations.

% \begin{figure}
% \vspace{-1.0em}
% \centering
% \centerline{\includegraphics[width=0.6\columnwidth]{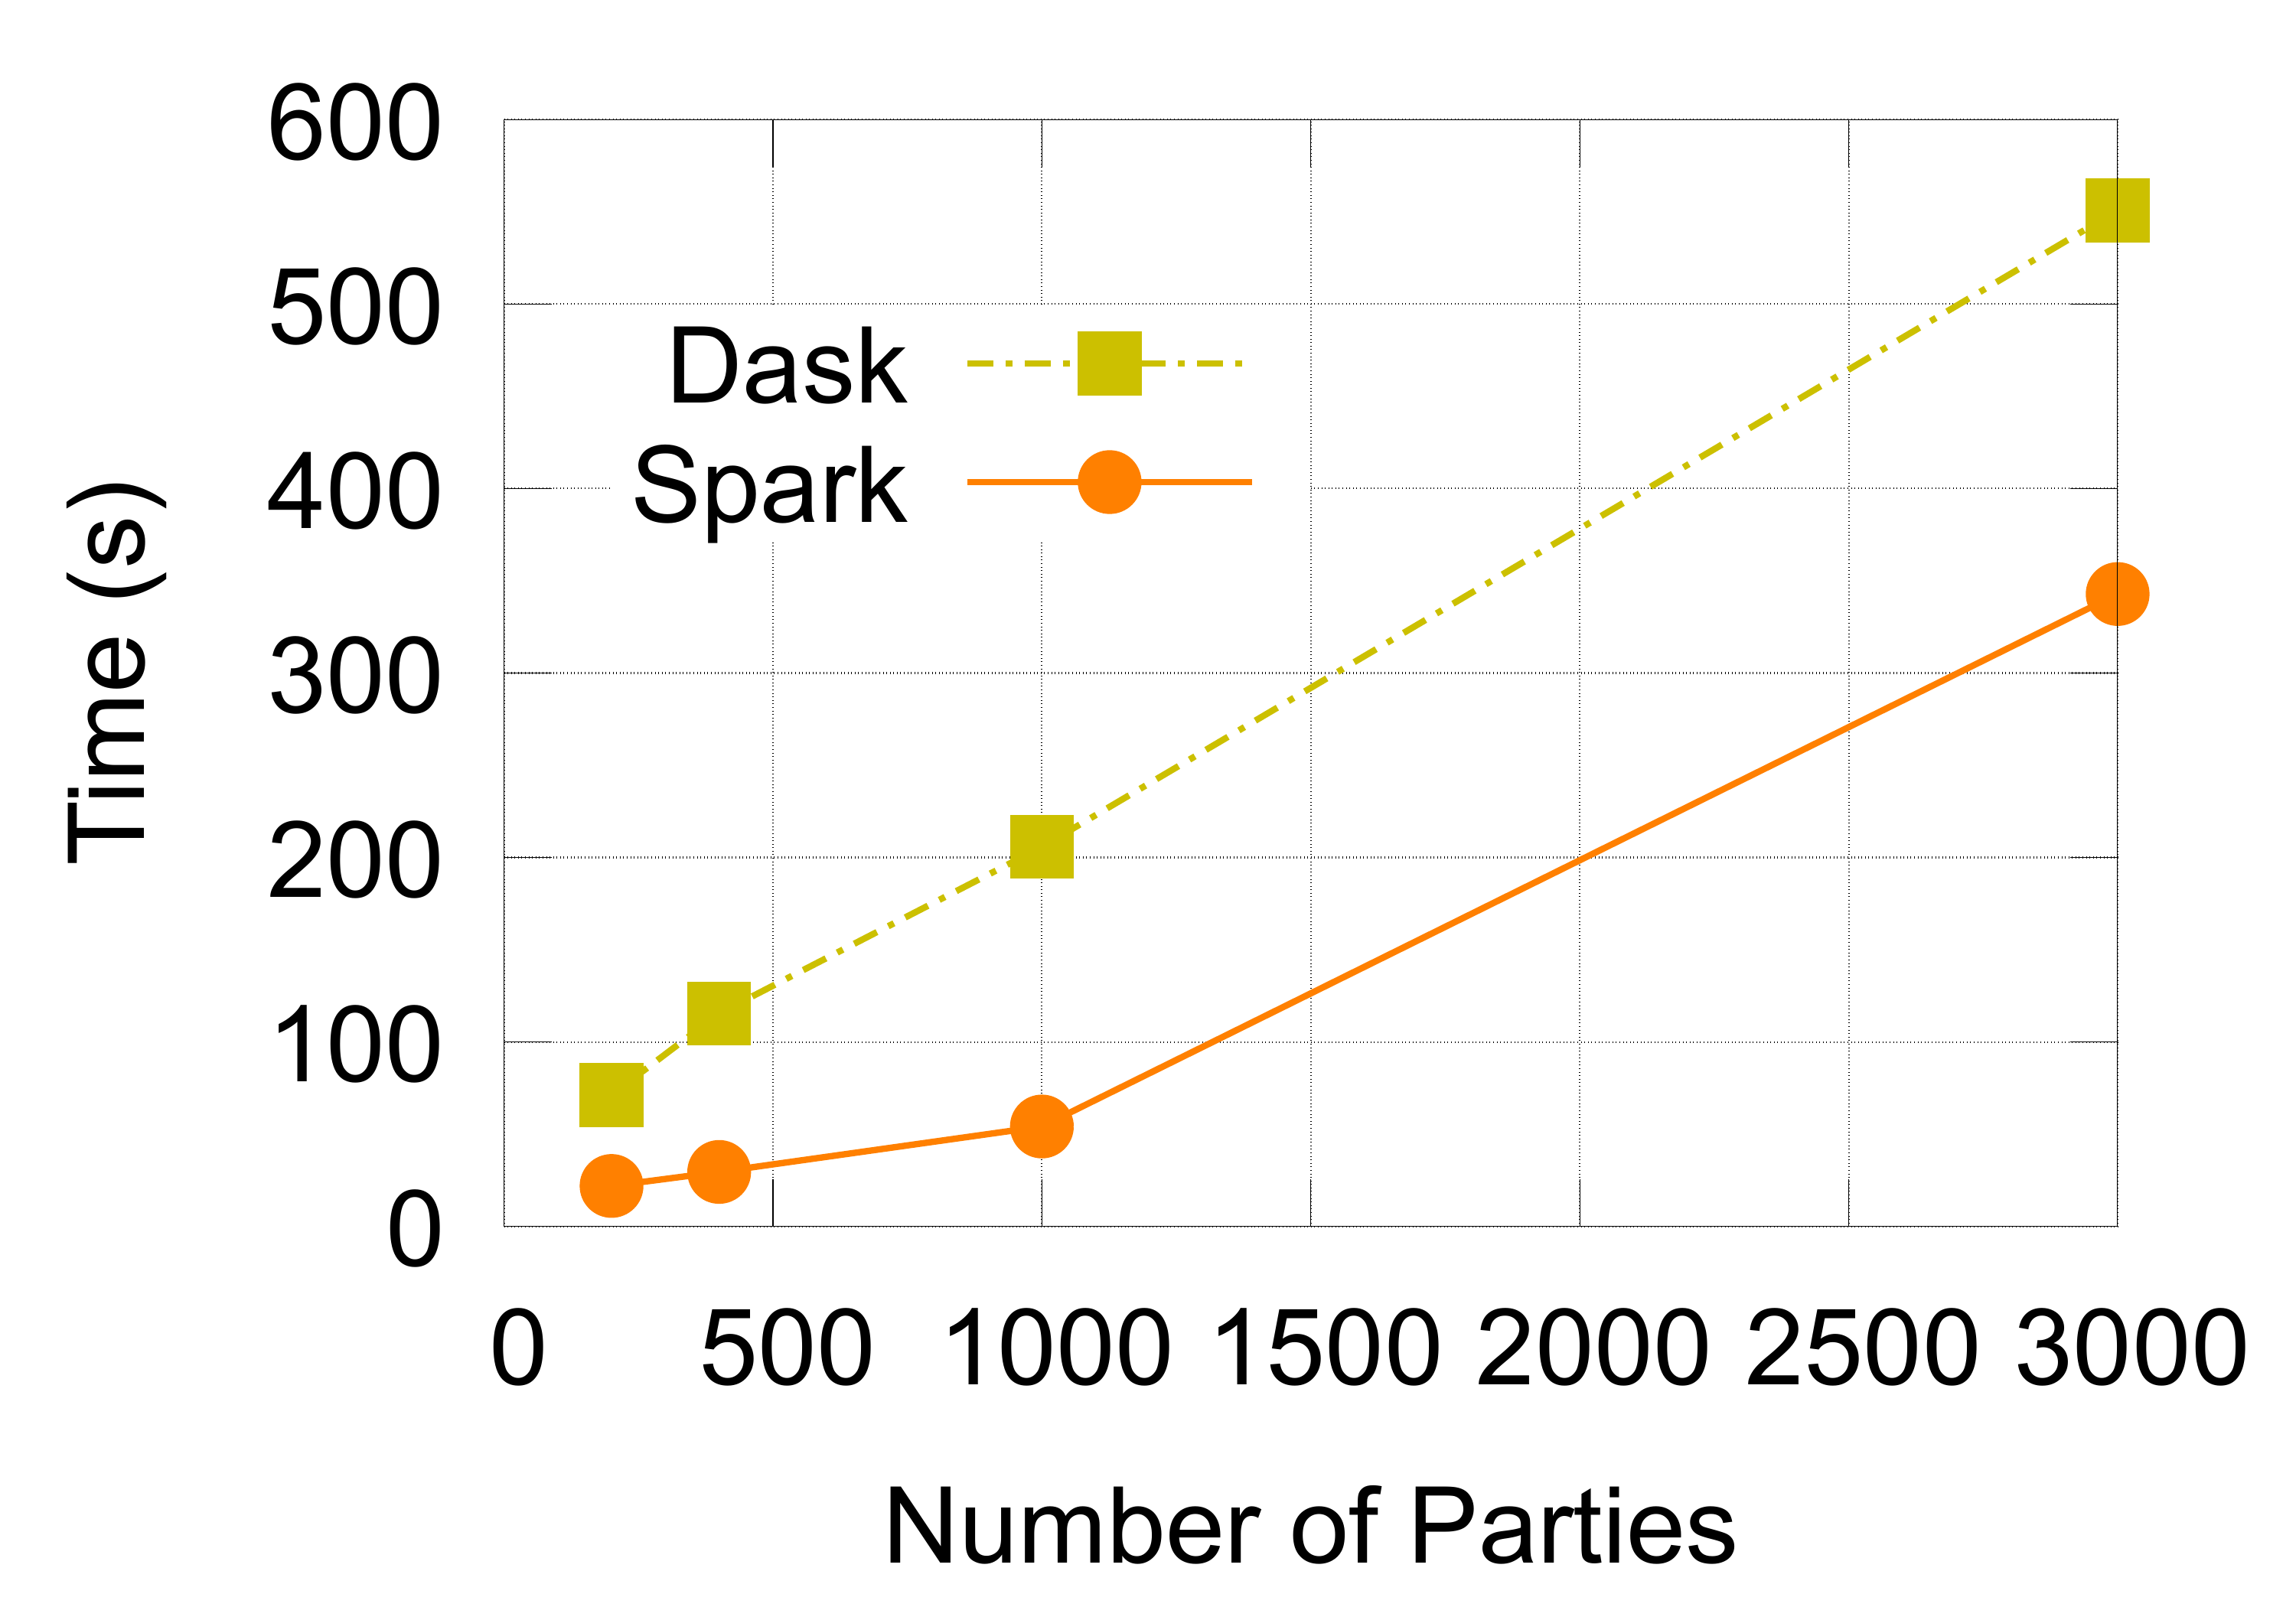}}
% \vspace{-12pt}
% \caption{Average aggregation time comparison for Dask and Spark-based method for Fedavg fusion algorithm on the Resnet50 model}
% \label{fig:dask_pyspark_resnet50}
% \vspace{-2.0em}
% \end{figure}
